# Supplementary material for: Anisotropic Etching of Graphite and Graphene in a Remote Hydrogen Plasma
Source: arXiv:1703.04762 ancillary file (2017-03-14)
Supplement: Supplementary file 1 [file supplementary.pdf]

Supplementary Information

# Anisotropic Etching of Graphite and Graphene in a Remote Hydrogen Plasma

D. Hug,[1] S. Zihlmann,[1] M. K. Rehmann,[1] Y. B. Kalyoncu,[1] T. N. Camenzind,[1] L. Marot,[1] K. Watanabe,[2] T. Taniguchi,[2] and D. M. Zumbuhl[1]

[1]*Department of Physics, University of Basel, CH-4056 Basel, Switzerland*

[2]*National Institute for Material Science, 1-1 Namiki, Tsukuba 305-0044, Japan*

## Plasma Furnace Setup

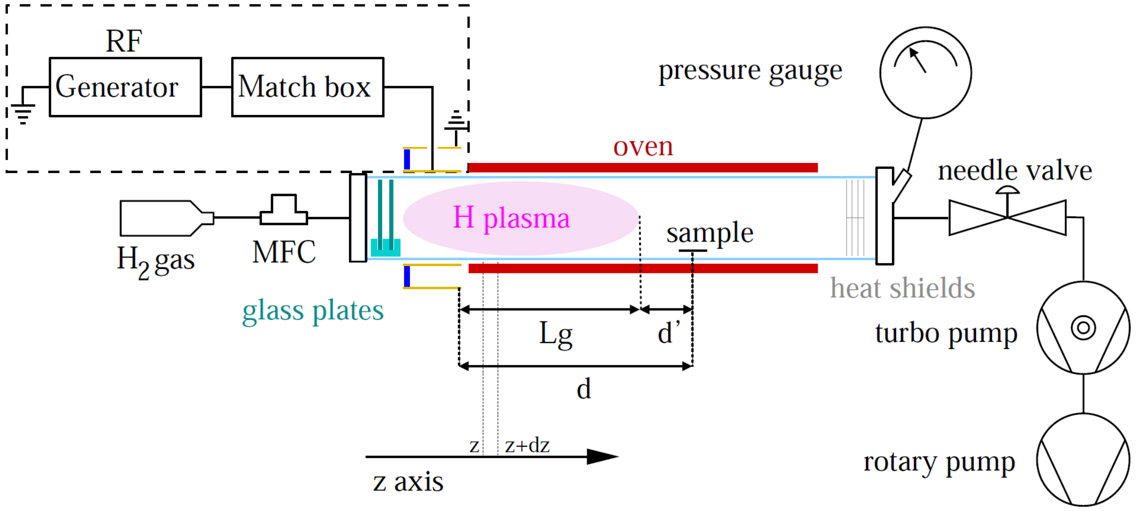


FIG. S1. **Setup** of the plasma furnace. The quartz tube has a length of ca. 1 m and a diameter of 80 mm (drawing not to scale).

## Direct and remote plasma region

In Figure S2, AFM scans acquired after exposure of natural graphite samples for 1 hour to a pure hydrogen (H) plasma at a power of 30 W depict the influence of the pressure and distance on the etching strength and type. For every pressure and distance combination a new graphite sample was fabricated as described in the main text. The matrix representation of the AFM scans of the complete set of investigated parameters remarkably demonstrates the transition from soft anisotropic etching (above or to the right of the cyan line) including only H atoms, to strong etching parameters (below or to the left of the cyan line) comprising also ions. The separation between the two regimes is based upon the size distribution of the hexagonal pits as ions are expected to induce defects acting as new etch sites throughout the whole exposure time. Lowering the pressure as well as decreasing the distance has the effect to increase the number of holes as well as the size distribution and depth of the etch pits, demonstrating an increase of the reactive particle density. On some of the AFM images, unintentional growth or deposition of some additional nanostructures such as worms or particles is seen, e.g. $d = 42\,\mathrm{cm}$ and $p = 1.4\,\mathrm{mbar}$ or $p = 0.7\,\mathrm{mbar}$.

For all AFM scans shown in Figure S2, the number of holes and their respective diameters

are evaluated and plotted in histograms shown in Figure S3, describing a comparable picture as the AFM topography scans. Again, not only the amount of holes but also the width of the diameter distribution shows a strong dependence on pressure and distance. As for the AFM scans, the remote (upper right) and the direct (lower left) plasma region can be distinguished using the widths of the distributions in the histograms. In the lower right panels we estimated the number of holes for each diameter to $> 12$ and the width of the diameter distribution to be at least 600 nm, since an exact investigation of the hole number and diameter was not feasible (see Figure S2).

The number of hexagons etched into the graphite surface as well as the width of the hole diameter distribution reflect the number of ions inducing defects on the graphitic surface, assuming a low intrinsic defect density on the surface of the graphite samples.

## Exponential decay of reactive particles

The number of holes (purple) and the width of the diameter distribution (orange) is shown in Figure S4 against the distance between the plasma edge and the sample, d$' = d - L_g$. For d$' < 0$ the sample is directly exposed to the glowing plasma, hence experiencing the impact of ions perforating the graphite surface with uncountable, several layers deep holes. For d$' > 0$ on the other hand, the hole number and the width of the hole distribution both appear to roughly decay exponentially with larger sample-plasma distance, with an 1/e decay length of $\sim 5$ cm extracted from a fit to an exponential (dashed lines).

The radical concentration is decaying exponentially when moving down the axis of the tube, and is given by [1, 2]

$$[H] = [H]_0 \cdot \exp\left(-a\sqrt{p}d'\right) \tag{1}$$

with sample-plasme edge distance $d'$, concentration $[H]_0$ at $d' = 0$, pressure $p$, and the geometrical factor $a$:

$$a = \sqrt{\frac{v_{therm}\gamma}{R \cdot D'}}. \tag{2}$$

Here, $v_{therm} = \sqrt{8k_BT/(\pi m)} \approx 2'750$ m/s is the molecular $H_2$ thermal velocity, with Boltzmann constant $k_B$, hydrogen mass $m$ and temperature $T$. The material dependent recombination coefficient [1, 2] of the radicals is $\gamma \approx 7.5 \cdot 10^{-4}$, $R = 4$ cm is the radius of the quartz tube and $D' = 7.39$ atm cm$^2$/s is the temperature dependent diffusion coefficient

[3, 4] taken here at $\sim 700\,\mathrm{K}$ from Ref. 3. Note the explicit pressure dependence of the decay length. Here, this results in a decay length of $\approx 12\,\mathrm{cm}$ at $p = 1\,\mathrm{mbar}$, which is consistent with our data. As mentioned in the main manuscript, the recombination of the radicals in the gas phase is expected to be irrelevant and the radicals only recombine at the surface of the quartz tube for the pressure range $p \sim 1\,\mathrm{mbar}$ used here.

## Raman measurements before and after plasma exposure

The influence of the H atoms on the graphene quality was further investigated by performing Raman measurements before, after 3 h and after 5 h of plasma exposure, as shown in Figure S5. To compare the Raman traces, we subtracted the background before normalizing the traces with the graphene G peak height at $\approx 1582cm^{-1}$. The Raman scans taken on the bare hBN substrate in panel D are normalized to the $SiO_2$ peak (not visible) to allow comparison. All Raman measurements presented in this work were acquired with a green laser with a wavelength of $\lambda = 533\,\mathrm{nm}$, where the bulk hBN $E_{2g}$ peak at $1366\,\mathrm{cm}^{-1}$ and the graphene D-peak at $1350\,\mathrm{cm}^{-1}$) are close to each other. Nevertheless, in many cases a weak D-peak can still be reliably extracted.

Panel D shows Raman spectra of the hBN flake before (yellow), after 3 h (blue) and after 5 h (red) of remote H plasma etching. The hBN $E_{2g}$ peak [5] shape, height and position does not significantly change, indicating no or only insignificant interaction of the hBN with the H plasma. Panel E shows Raman spectra acquired on bulk graphene, again before (yellow), after 3 h (blue) and after 5 h (red) of H plasma etching. We did not observe a D-peak in the bulk of the graphene flakes even after 15 h of plasma etching (not shown), indicating no induction of defects or hydrogenation of our samples [6, 7]. Note that after the end of the plasma exposure, the samples are annealed in vacuum while the oven is cooling down from process temperature to room temperature.

Significant information about the type and quality of edge can in principle be obtained from Raman spectra of the graphene edge [8]. However, care needs to be taken to not overheat and possibly reconstruct or otherwise change the edge with the laser [9] when illuminating the graphene edge on $SiO_2$ at a laser power of 1.5 mW or more. Our spectra do not meet these low power requirements. The damage threshold for graphene on hBN is

not known, and study of these effects goes beyond the scope of this work.

### A. REFERENCES

---


[1] R. K. Grubbs and S. M. George, *Attenuation of hydrogen radicals traveling under flowing gas conditions through tubes of different materials*, Journal of Vacuum Science & Technology A: Vacuum, Surfaces, and Films **24**, 486 (2006).

[2] Y.C. Kim and M. Boudart, *Recombination of O, N and H atoms on Silica: Kinetics and Mechanism*, Langmuir page 2999 (May 1991).

[3] K.M. Sancier and H. Wise, *Diffusion and Heterogeneous Reaction. XI. Diffusion Coefficient Measurements for Gas Mixture of Atomic and Molecular Hydrogen*, Journal of Chemical Physics **51**, 1434 (1969).

[4] Stanley Weissman and EA Mason, *Estimation of the mutual diffusion coefficient of hydrogen atoms and molecules*, The Journal of Chemical Physics **36**, 794 (1962).

[5] R. Geick, C. H. Perry, and G. Rupprecht, *Normal modes in hexagonal boron nitride*, Physical Review **146**, 543 (1966).

[6] A. C. Ferrari, J. C. Meyer, V. Scardaci, C. Casiraghi, M. Lazzeri, F. Mauri, S. Piscanec, D. Jiang, K. S. Novoselov, S. Roth, and A. K. Geim, *Raman Spectrum of Graphene and Graphene Layers*, Physical Review Letters **97** (October 2006).

[7] D. C. Elias, R. R. Nair, T. M. G. Mohiuddin, S. V. Morozov, P. Blake, M. P. Halsall, A. C. Ferrari, D. W. Boukhvalov, M. I. Katsnelson, and A. K. Geim, *Control of graphene's properties by reversible hydrogenation: evidence for graphane*, Science **323**, 610 (2009).

[8] B. Krauss, P. Nemes-Incze, V. Skakalova, L. P. Biro, K. von Klitzing, and J.H. Smet, *Raman Scattering at Pure Graphene Zigzag Edges*, Nano Letters **10**, 4544–4548 (November 2010).

[9] M. Begliarbekov, K.I. Sasaki, O. Sul, E.H. Yang, and St. Strauf, *Optical Control of Edge Chirality in Graphene*, Nano Letters **11**, 4874 (November 2011).

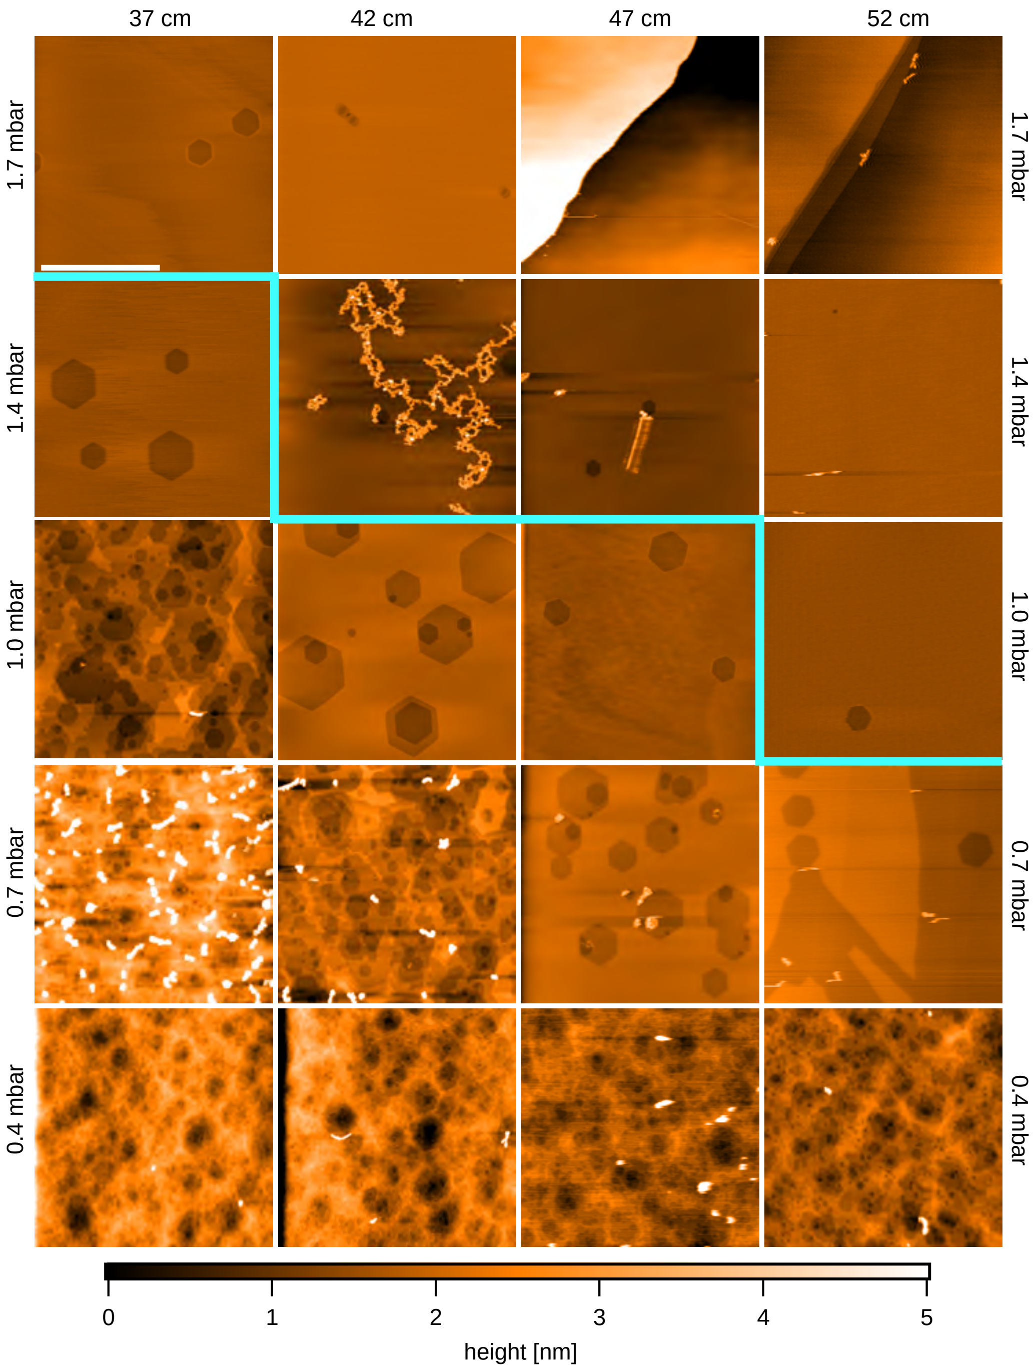


FIG. S2. **Distance and pressure dependence of graphite plasma exposure.** AFM topography scans at all parameters investigated in Figure 1E in the main paper. All AFM images are $2 \times 2\,\mu\mathrm{m}^2$ in size. The cyan curve marks the transition from the remote (upper right) to the direct (lower left) plasma region. On some surfaces, particles are visible which probably are amorphous carbon residues, either grown or deposited during the etching process (see AFM scans for $p = 0.7\,\mathrm{mbar}$ and $d = 37\,\mathrm{cm}$ or $p = 1.4\,\mathrm{mbar}$ and $d = 42\,\mathrm{cm}$).

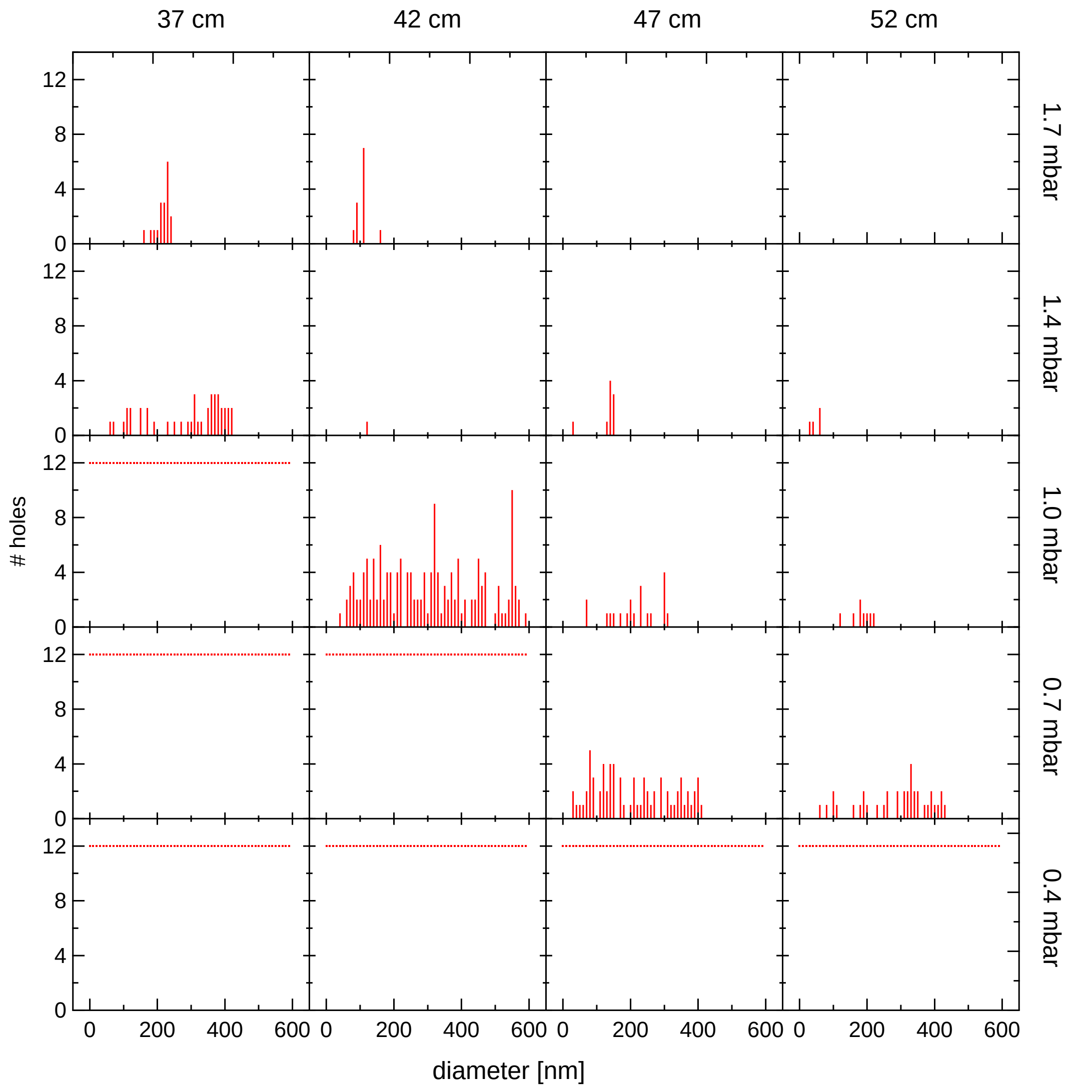


FIG. S3. **Distance and pressure dependence of graphite plasma exposure.** Histograms (10 nm bin size) showing the number of holes for all pressure and distance parameters corresponding to Figure S2, obtained from $10 \times 10\,\mu m^2$ AFM scans. For AFM scans of strongly etched surfaces, we plot 12 holes for every hole diameter.

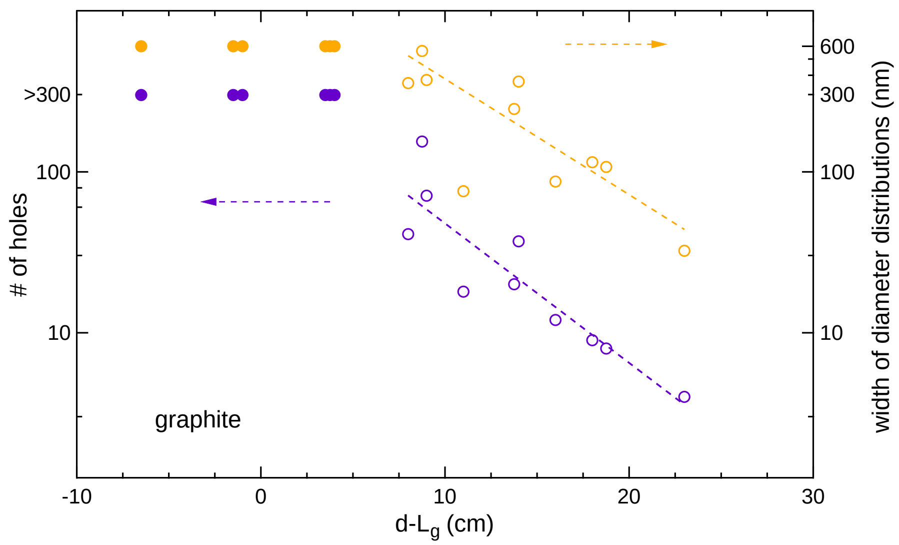


FIG. S4. Number of holes (purple, left axis) and width of diameter distribution (orange, right axis) as a function of effective distance $d' = d - L_g$.

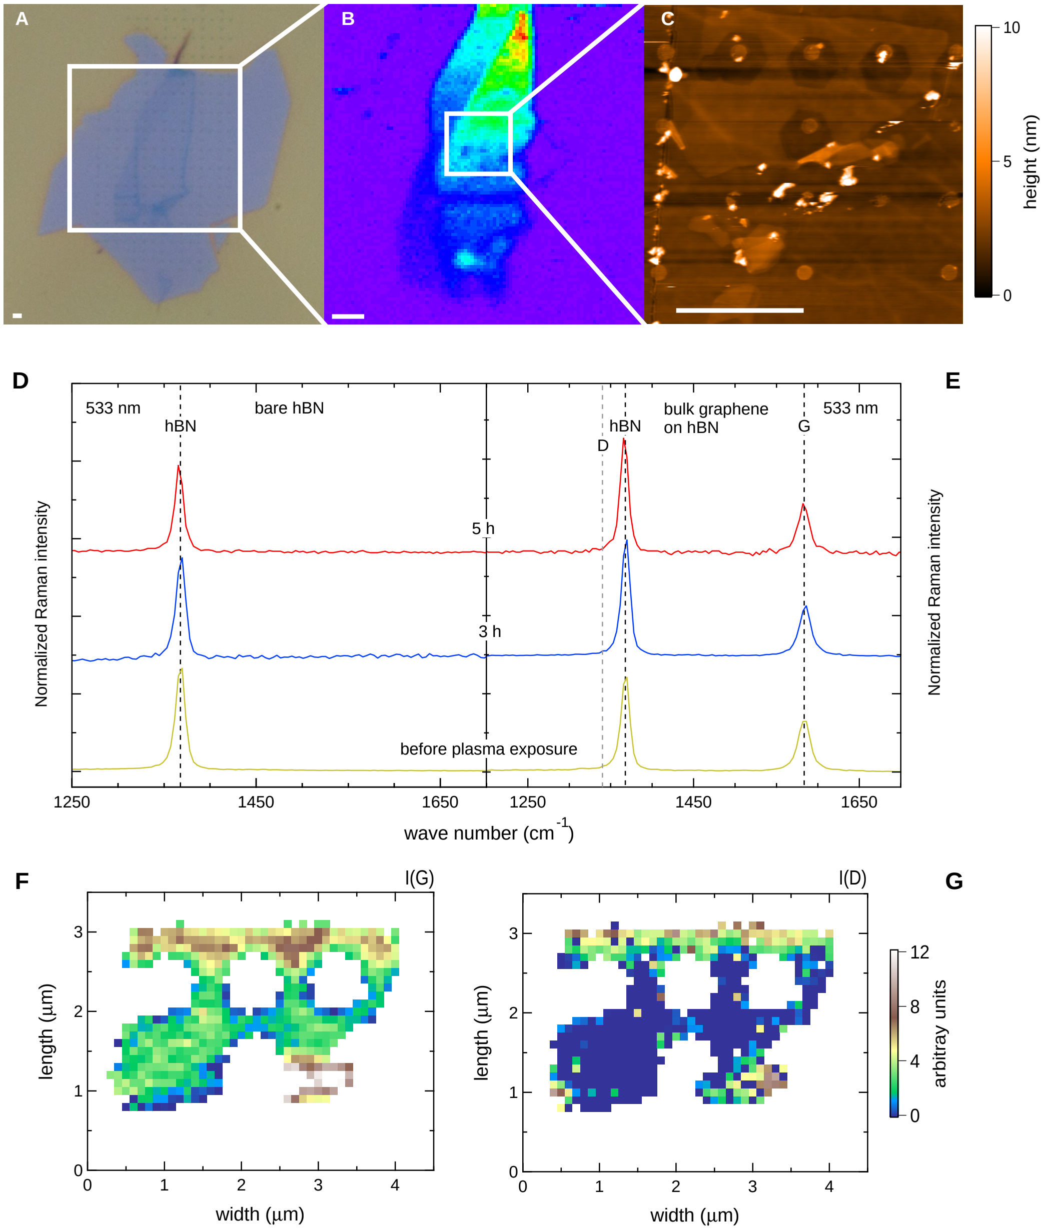


FIG. S5. **Raman spectra and spatially resolved Raman scans of the hBN sample in the main paper.** Panel A: optical image of a graphene on hBN sample. Panel B: Raman map of the 2D peak of the same graphene flake before H plasma exposure. Panel C: AFM topography scan showing the region where the Raman single spectra were taken. The scale bars in Panel A to C are 2 $\mu$m. Panel D and E: Raman spectra of the bare hBN flake (panel D) and bulk graphene on hBN (panel E) before (yellow), after 3 h (blue) and after 5 h (red) of remote plasma exposure. The Raman spectra are vertically shifted for clarity. Panel F and G: 2D maps of the G peak (panel F) and D peak (panel G) of the flake region shown in panel C.
